# Supplementary material for: Universal Semi-Supervised Semantic Segmentation
Source: arXiv:1811.10323 source file (2019-09-24)
Supplement: Supplementary file 1 [file qualt.tex]

\begin{figure*}
\vspace{-0.5em}
\centering
        \begin{subfigure}[b]{0.248\textwidth}
                \centering
                \includegraphics[width=\linewidth]{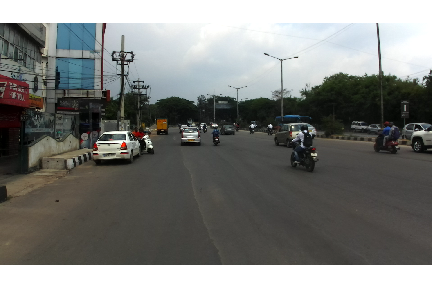}
                \vspace{-2em}
                % \caption{\label{fig:anue_image}}        
                
        \end{subfigure}\hfill
        \begin{subfigure}[b]{0.248\textwidth}
                \centering
                \includegraphics[width=\linewidth]{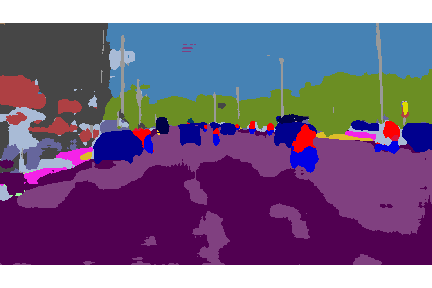}
                \vspace{-2em}
                % \caption{\label{fig:anue_bad}}
        \end{subfigure}\hfill
        \begin{subfigure}[b]{0.248\textwidth}
                \centering
                \includegraphics[width=\linewidth]{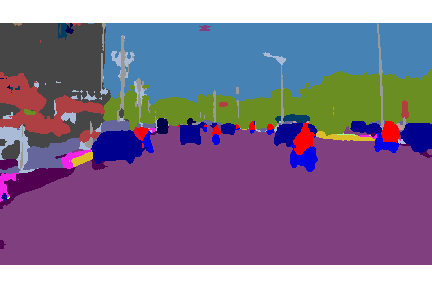}
                \vspace{-2em}
                % \caption{\label{fig:anue_good}}
        \end{subfigure}\hfill
        \begin{subfigure}[b]{0.248\textwidth}
                \centering
                \includegraphics[width=\linewidth]{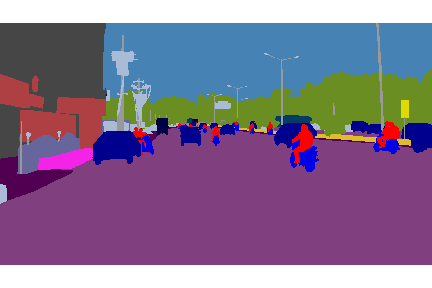}
                \vspace{-2em}
                % \caption{\label{fig:anue_label}}         
                
        \end{subfigure}\hfill
        ~
        \begin{subfigure}[b]{0.248\textwidth}
                \centering
                \includegraphics[width=\linewidth]{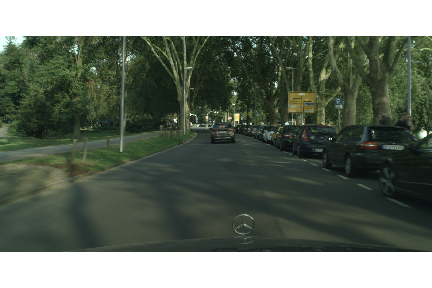}
                % \vspace{-2.5em}
                % \caption{\label{fig:cs_image}}
        \end{subfigure}\hfill
        \begin{subfigure}[b]{0.248\textwidth}
                \centering
                \includegraphics[width=\linewidth]{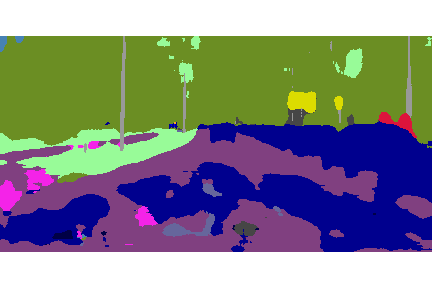}
                % \vspace{-2.5em}
                % \caption{\label{fig:cs_bad}}
        \end{subfigure}\hfill
        \begin{subfigure}[b]{0.248\textwidth}
                \centering
                \includegraphics[width=\linewidth]{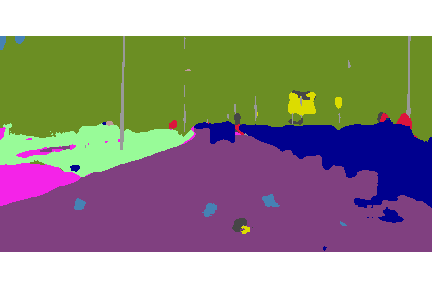}
                % \vspace{-2.5em}
                % \caption{\label{fig:cs_good}}
        \end{subfigure}\hfill
        \begin{subfigure}[b]{0.248\textwidth}
                \centering
                \includegraphics[width=\linewidth]{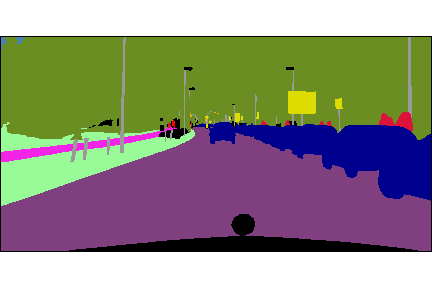}
                % \vspace{-2.5em}
                % \caption{\label{fig:cs_label}}
        \end{subfigure}\hfill
        % \caption{}
        ~
        \begin{subfigure}[b]{0.248\textwidth}
                \centering
                \includegraphics[width=\linewidth]{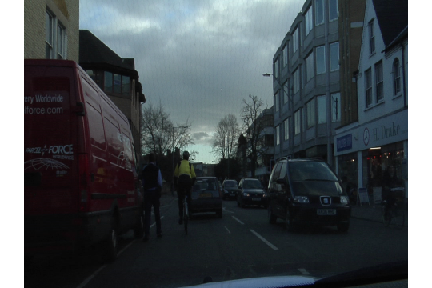}
                \vspace{-1.5em}
                \caption{Original Image\label{fig:cvd_image}}
        \end{subfigure}\hfill
        \begin{subfigure}[b]{0.248\textwidth}
                \centering
                \includegraphics[width=\linewidth]{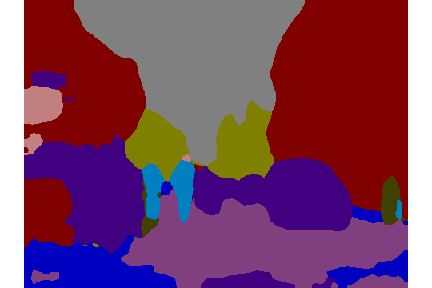}
                \vspace{-1.5em}
                \caption{Without Entropy Module\label{fig:cvd_bad}}
        \end{subfigure}\hfill
        \begin{subfigure}[b]{0.248\textwidth}
                \centering
                \includegraphics[width=\linewidth]{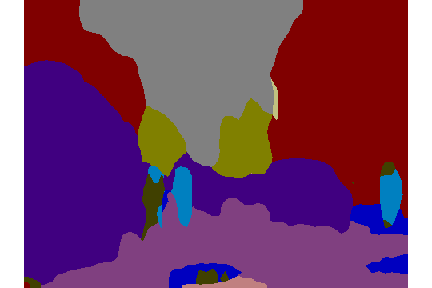}
                \vspace{-1.5em}
                \caption{With Entropy Module\label{fig:cvd_good}}
        \end{subfigure} \hfill
        \begin{subfigure}[b]{0.248\textwidth}
                \centering
                \includegraphics[width=\linewidth]{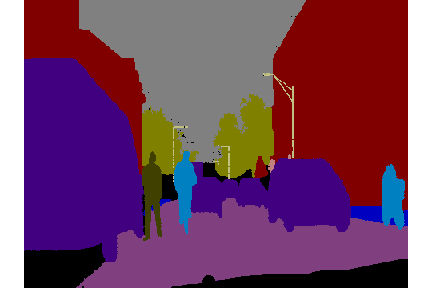}
                \vspace{-1.5em}
                \caption{Ground Truth Segmentation\label{fig:cvd_label}}
        \end{subfigure}\hfill
        \captionsetup{width=0.95\textwidth}
        \caption{Qualitative examples from each dataset training with and without the proposed entropy regularization module. The first row shows example from IDD dataset, second row from Cityscapes and the third from the CamVid dataset.}
        \label{fig:qualitative}
        % \bigskip
        % \vspace{-1em}
\end{figure*}
