# Supplementary material for: Universal Semi-Supervised Semantic Segmentation
Source: arXiv:1811.10323 source file (2019-09-24)
Supplement: Supplementary file 4 [file qualt_cs.tex]

% \section{Qualitative Examples}
% Some more qualitative examples from cityscapes, IDD and CamVid datasets to compare the performance of the \textit{Univ-full} and the \textit{Univ-basic} models. 
\begin{figure*}[!ht]

\centering
        
        \begin{subfigure}[b]{0.248\textwidth}
                \centering
                \includegraphics[width=\linewidth]{qualt_figs/CS_image_306.png}
                \vspace{-1em}
                % \caption{\label{fig:cs_image}}        
                
        \end{subfigure}\hfill
        \begin{subfigure}[b]{0.248\textwidth}
                \centering
                \includegraphics[width=\linewidth]{qualt_figs/CS_bad_pred_306.png}
                \vspace{-1em}
                % \caption{\label{fig:cs_bad}}
        \end{subfigure}\hfill
        \begin{subfigure}[b]{0.248\textwidth}
                \centering
                \includegraphics[width=\linewidth]{qualt_figs/CS_good_pred_306.png}
                \vspace{-1em}
                % \caption{\label{fig:cs_good}}
        \end{subfigure}\hfill
        \begin{subfigure}[b]{0.248\textwidth}
                \centering
                \includegraphics[width=\linewidth]{qualt_figs/CS_label_306.png}
                \vspace{-1em}
                % \caption{\label{fig:cs_label}}         
                
        \end{subfigure}\hfill
        \vspace{-1em}
        ~
        % \vspace{2em}
        \begin{subfigure}[b]{0.248\textwidth}
                \centering
                \includegraphics[width=\linewidth]{qualt_figs/CS_image_490.png}
                \vspace{-1em}
                % \caption{\label{fig:cs_image}}
        \end{subfigure}\hfill
        \begin{subfigure}[b]{0.248\textwidth}
                \centering
                \includegraphics[width=\linewidth]{qualt_figs/CS_bad_pred_490.png}
                \vspace{-1em}
                % \caption{\label{fig:cs_bad}}
        \end{subfigure}\hfill
        \begin{subfigure}[b]{0.248\textwidth}
                \centering
                \includegraphics[width=\linewidth]{qualt_figs/CS_good_pred_490.png}
                \vspace{-1em}
                % \caption{\label{fig:cs_good}}
        \end{subfigure}\hfill
        \begin{subfigure}[b]{0.248\textwidth}
                \centering
                \includegraphics[width=\linewidth]{qualt_figs/CS_label_490.png}
                \vspace{-1em}
                % \caption{\label{fig:cs_label}}
        \end{subfigure}\hfill
        % \caption{}
        \vspace{-1em}
        ~
        % \vspace{2em}
        \begin{subfigure}[b]{0.248\textwidth}
                \centering
                \includegraphics[width=\linewidth]{qualt_figs/CS_image_287.png}
                \vspace{-1em}
                \caption{Original Image\label{fig:cs_image}}
        \end{subfigure}\hfill
        \begin{subfigure}[b]{0.248\textwidth}
                \centering
                \includegraphics[width=\linewidth]{qualt_figs/CS_bad_pred_287.png}
                \vspace{-1em}
                \caption{Without Entropy Module\label{fig:cs_bad}}
        \end{subfigure}\hfill
        \begin{subfigure}[b]{0.248\textwidth}
                \centering
                \includegraphics[width=\linewidth]{qualt_figs/CS_good_pred_287.png}
                \vspace{-1em}
                \caption{With Entropy Module\label{fig:cs_good}}
        \end{subfigure} \hfill
        \begin{subfigure}[b]{0.248\textwidth}
                \centering
                \includegraphics[width=\linewidth]{qualt_figs/CS_label_287.png}
                \vspace{-1em}
                \caption{Ground Truth Segmentation\label{fig:cs_label}}
        \end{subfigure}\hfill
        \captionsetup{width=0.95\textwidth}
        \caption{Qualitative examples from the cityscapes dataset with and without the proposed entropy regularization module, when trained on a universal model on CS+CamVid.}
        \label{fig:qualitative_cs}
        % \bigskip
        \vspace{-1em}
\end{figure*}
